# Supplementary material for: ECtHR-PCR: A Dataset for Precedent Understanding and Prior Case Retrieval in the European Court of Human Rights
Source: arXiv:2404.00596 source file (2024-03-31)
Supplement: Supplementary file 1 [file appendix.tex]

\section{Distribution of Outgoing citations}
Fig. \ref{out_cit} displays the distribution of outgoing citations of all documents.

\begin{figure}
    \centering
    \includegraphics[width = 0.5\textwidth]{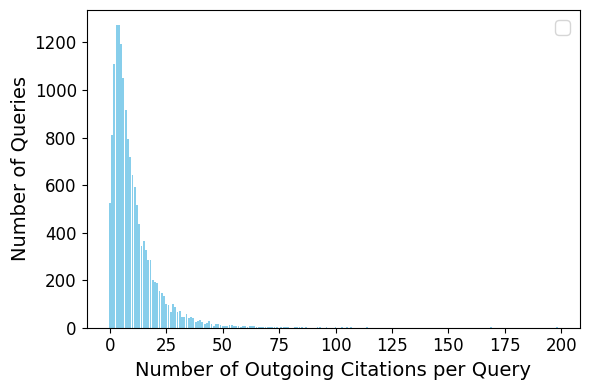}
    \caption{Distribution of outgoing citations per query.}
    \label{out_cit}
\end{figure}

\section{Distribution of Incoming citations}
Figure \ref{inc_cit} illustrates the distribution of incoming citations for all documents, indicating the number of times each document has been referenced by other cases. Among the analyzed documents, approximately 6k cases have not received any citations. Notably, around 1.5k of these cases belong to the last 5 years, representing more than 50\% of the cases in this period. It is expected that recent cases may not have been cited yet, as it takes time for them to gain attention and recognition within the legal community. On the other hand, approximately 1.7k cases have been cited exactly once, while the remaining cases have received multiple citations.

The frequency of incoming citations serves as an indicator of the influence and relevance of a case within the legal domain. Cases that have been cited multiple times are likely to contain valuable legal arguments, reasoning, or precedents that have been widely recognized and referenced by other cases. Therefore, considering citation frequency as a signal can be beneficial for modeling relevance in prior case retrieval and should be considered in future. %By incorporating this signal into retrieval models, we can prioritize and retrieve cases that have a higher impact and are more relevant to the query case.
\begin{figure}
    \centering
    \includegraphics[width = 0.5\textwidth]{images/dist_inc.png}
    \caption{Distribution of documetns based on incoming citations. (expressed in log scale)}
    \label{inc_cit}
\end{figure}

\section{Hierarchical Encoder}
\label{arch}
We follow the greedy packing strategy to obtain the input $x = \{x_1, x_2, \ldots, x_m\}$ where $x_i = \{x_{i1}, x_{i2}, \ldots, x_{in}\}$. ${x_i}$, ${x_{ij}}$, m and n denote $i^\text{th}$ packet, $j^\text{th}$ token in $i^\text{th}$ packet, number of packets, number of tokens in $i^\text{th}$ packet respectively. 

\noindent \textbf{Token encoding layer} We use BERT encoders to obtain token-level representations $z_i = \{z_{i1}, z_{i2}, \ldots, z_{in}\}$ for each token in every packet $x_i = \{x_{i1}, x_{i2}, \ldots, x_{in}\}$. 

\noindent \textbf{Token attention layer} 
%We utilize an attention mechanism to identify the salient tokens in each packet. 
We obtain the representation for each packet by aggregating their token-level representations using attention as follows:
\begin{equation}
    u_{it} = \tanh(W_w z_{it} + b_w )  
\end{equation}
\begin{equation}
    \alpha_{it} = \frac{\exp(u_{it}u_w)}{\sum_t \exp(u_{it}u_w)}  
~~\&~~
    f_i = \sum_{t=1}^n \alpha_{it}z_{it}
\label{att}
\end{equation}
where $W_w$,$b_w$ and $u_w$ are trainable parameters and $\alpha_{it}$ represents the importance of $t^\text{th}$ token in the $i^\text{th}$ packet. 

Thus we obtain the representations for the input packets as $f= \{f_1, f_2, \ldots, f_m\}$.

\noindent \textbf{Packet encoding} 
Given the packet vectors $f$ from token attention layer, we pass them through a bi-directional GRU to obtain context-aware packet representations $g = \{g_1, g_2, \ldots, g_m\}$.

\noindent \textbf{Packet attention layer} Finally, we aggregate packet representations $g$ into final dense representation of the input $c$ using  attention as follows.
\begin{equation}
    v_{i} = \tanh(W_s g_i + b_s )  
\end{equation}
\begin{equation}
    \beta_i = \frac{\exp(v_iv_s)}{\sum_i \exp(v_i v_s)}
~~\&~~
    c = \sum_{i=1}^m \beta_i g_i
\label{att}
\end{equation}
%where $W_s$,$b_s$ and $v_s$ are trainable parameters and $\beta_i$ represents the importance of $i^\text{th}$ packet.

\section{Implementation Details}
\label{imp_details}
 $k_1$ and $b$ are hyperparameters in BM25 that favors high tf scores and penalizing long documents respectively and $K_1$ evaluated in the range[0, 3] and b in [0, 1] to pick the best value based ont he validation set. For all our dense models, we use LegalBERT as backbone which produce word embeeding size of size 768. Our word level attention context vector size is 300. The sentence level GRU encoder dimension is 200, thus giving a bidirectional embedding of size 400, and a sentence level attention vector dimension of 200. We use 4 queries in a batch with 1 positive and 7 negative per query, resulting in 32 cases per batch. The model is optimized end- to-end using Adam \cite{kingma2014adam}.  We determine the best learning rate using a grid search on the validation set and use early stopping based on the development set based on Recall@1000 score.

\section{Performance across cases of different alleged articles}
To obtain list of allegation articles, we first parse the conclusions section in the case judgement document. After noticing some alleged articles being mentioned in the texts were missing in the conclusion section, to improve quality, we also parsed section headers under the law section in the judgement. We report the average of Recall@1000 values across cases which involve a specific allegation article in Fig. \ref{fig:alleg}. We observe complementarity between BM25 and DR-Rand across different articles, in both frequent and rare article settings. Hence we should leverage a combination of both of these methods where dense methods capture semantic nuances from contextual understanding where as BM25 keyword matching mechanism deals effectively with discriminative and rare legal terms present in the texts. However, this need to be understood in the background of multiplicity of allegations involved under case and we do not have a clear signal to relate each cited document to specific article and leave that for future investigation.

\begin{figure*}
    \centering
    \includegraphics[width=0.8\textwidth]{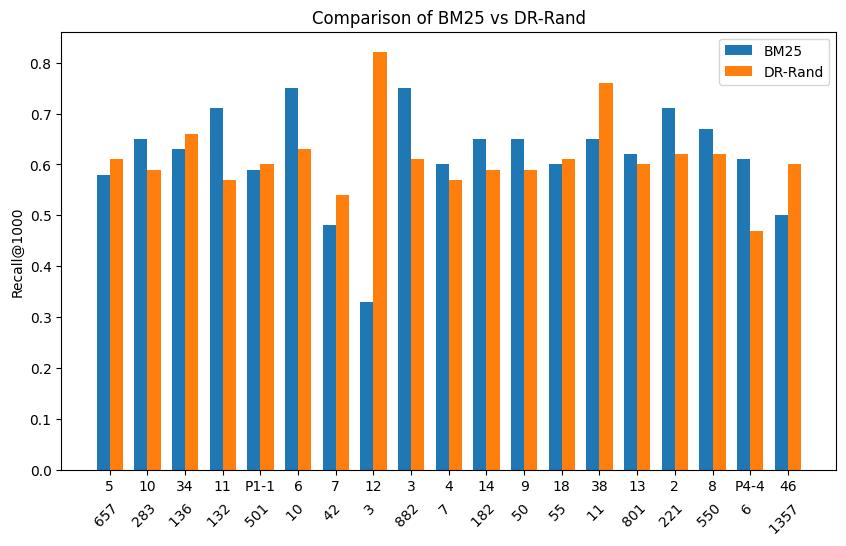}
    \caption{Recall@1000 scores for cases with different allegation articles. Horizontal text on X-axis indicates different articles and the inclined text indicates number of documents cooresponding to that alleged article.}
    \label{fig:alleg}
\end{figure*}
